# Supplementary material for: Hierarchical Conversational Preference Elicitation with Bandit Feedback
Source: arXiv:2209.06129 source file (2022-09-06)
Supplement: Supplementary file 1 [file 9_appendix.tex]

\appendix
\section{Proof of Theorem~\ref{lemma:T_k}}
\newpage
